# Supplementary material for: Scalable Dual Coordinate Descent for Kernel Methods
Source: arXiv:2406.18001 source file (2024-06-26)
Supplement: Supplementary file 1 [file appendix.tex]

\pagebreak

\section{Additional Experiments}

Below are the remaining experiments results of the performance experiments, including block-dual coordinate descent and dual coordinate descent experiments.

\subsection{Running Time Breakdown}

\subsection{Strong Scaling}
This section contains additional running time breakdown and strong scaling experiments.

\subsubsection{BDCD}

\begin{figure*}
  \centering
  \setkeys{Gin}{width=1\linewidth}
  \begin{subfigure}[t]{0.32\textwidth}
    \includegraphics{figures/ridge/general/Cabdcd_Newsbinary_linear_b1_Max.pdf}
    \caption{news20.binary, Batch size = 1, linear}
  \end{subfigure}\hfill
  \begin{subfigure}[t]{0.32\textwidth}
    \includegraphics{figures/ridge/general/Cabdcd_Newsbinary_linear_b2_Max.pdf}
    \caption{news20.binary, Batch size = 2, linear}
  \end{subfigure}\hfill
  \begin{subfigure}[t]{0.32\textwidth}
    \includegraphics{figures/ridge/general/Cabdcd_Newsbinary_linear_b4_Max.pdf}
    \caption{news20.binary, Batch size = 4, linear}
  \end{subfigure}\hfill

    \setkeys{Gin}{width=1\linewidth}
  \begin{subfigure}[t]{0.32\textwidth}
    \includegraphics{figures/ridge/general/Cabdcd_Newsbinary_poly_b1_Max.pdf}
    \caption{news20.binary, Batch size = 1, poly}
  \end{subfigure}\hfill
  \begin{subfigure}[t]{0.32\textwidth}
    \includegraphics{figures/ridge/general/Cabdcd_Newsbinary_poly_b2_Max.pdf}
    \caption{news20.binary, Batch size = 2, poly}
  \end{subfigure}\hfill
  \begin{subfigure}[t]{0.32\textwidth}
    \includegraphics{figures/ridge/general/Cabdcd_Newsbinary_poly_b4_Max.pdf}
    \caption{news20.binary, Batch size = 4, poly}
  \end{subfigure}\hfill

    \setkeys{Gin}{width=1\linewidth}
  \begin{subfigure}[t]{0.32\textwidth}
    \includegraphics{figures/ridge/general/Cabdcd_Newsbinary_gauss_b1_Max.pdf}
    \caption{news20.binary, Batch size = 1, gauss}
  \end{subfigure}\hfill
  \begin{subfigure}[t]{0.32\textwidth}
    \includegraphics{figures/ridge/general/Cabdcd_Newsbinary_gauss_b2_Max.pdf}
    \caption{news20.binary, Batch size = 2, gauss}
  \end{subfigure}\hfill
  \begin{subfigure}[t]{0.32\textwidth}
    \includegraphics{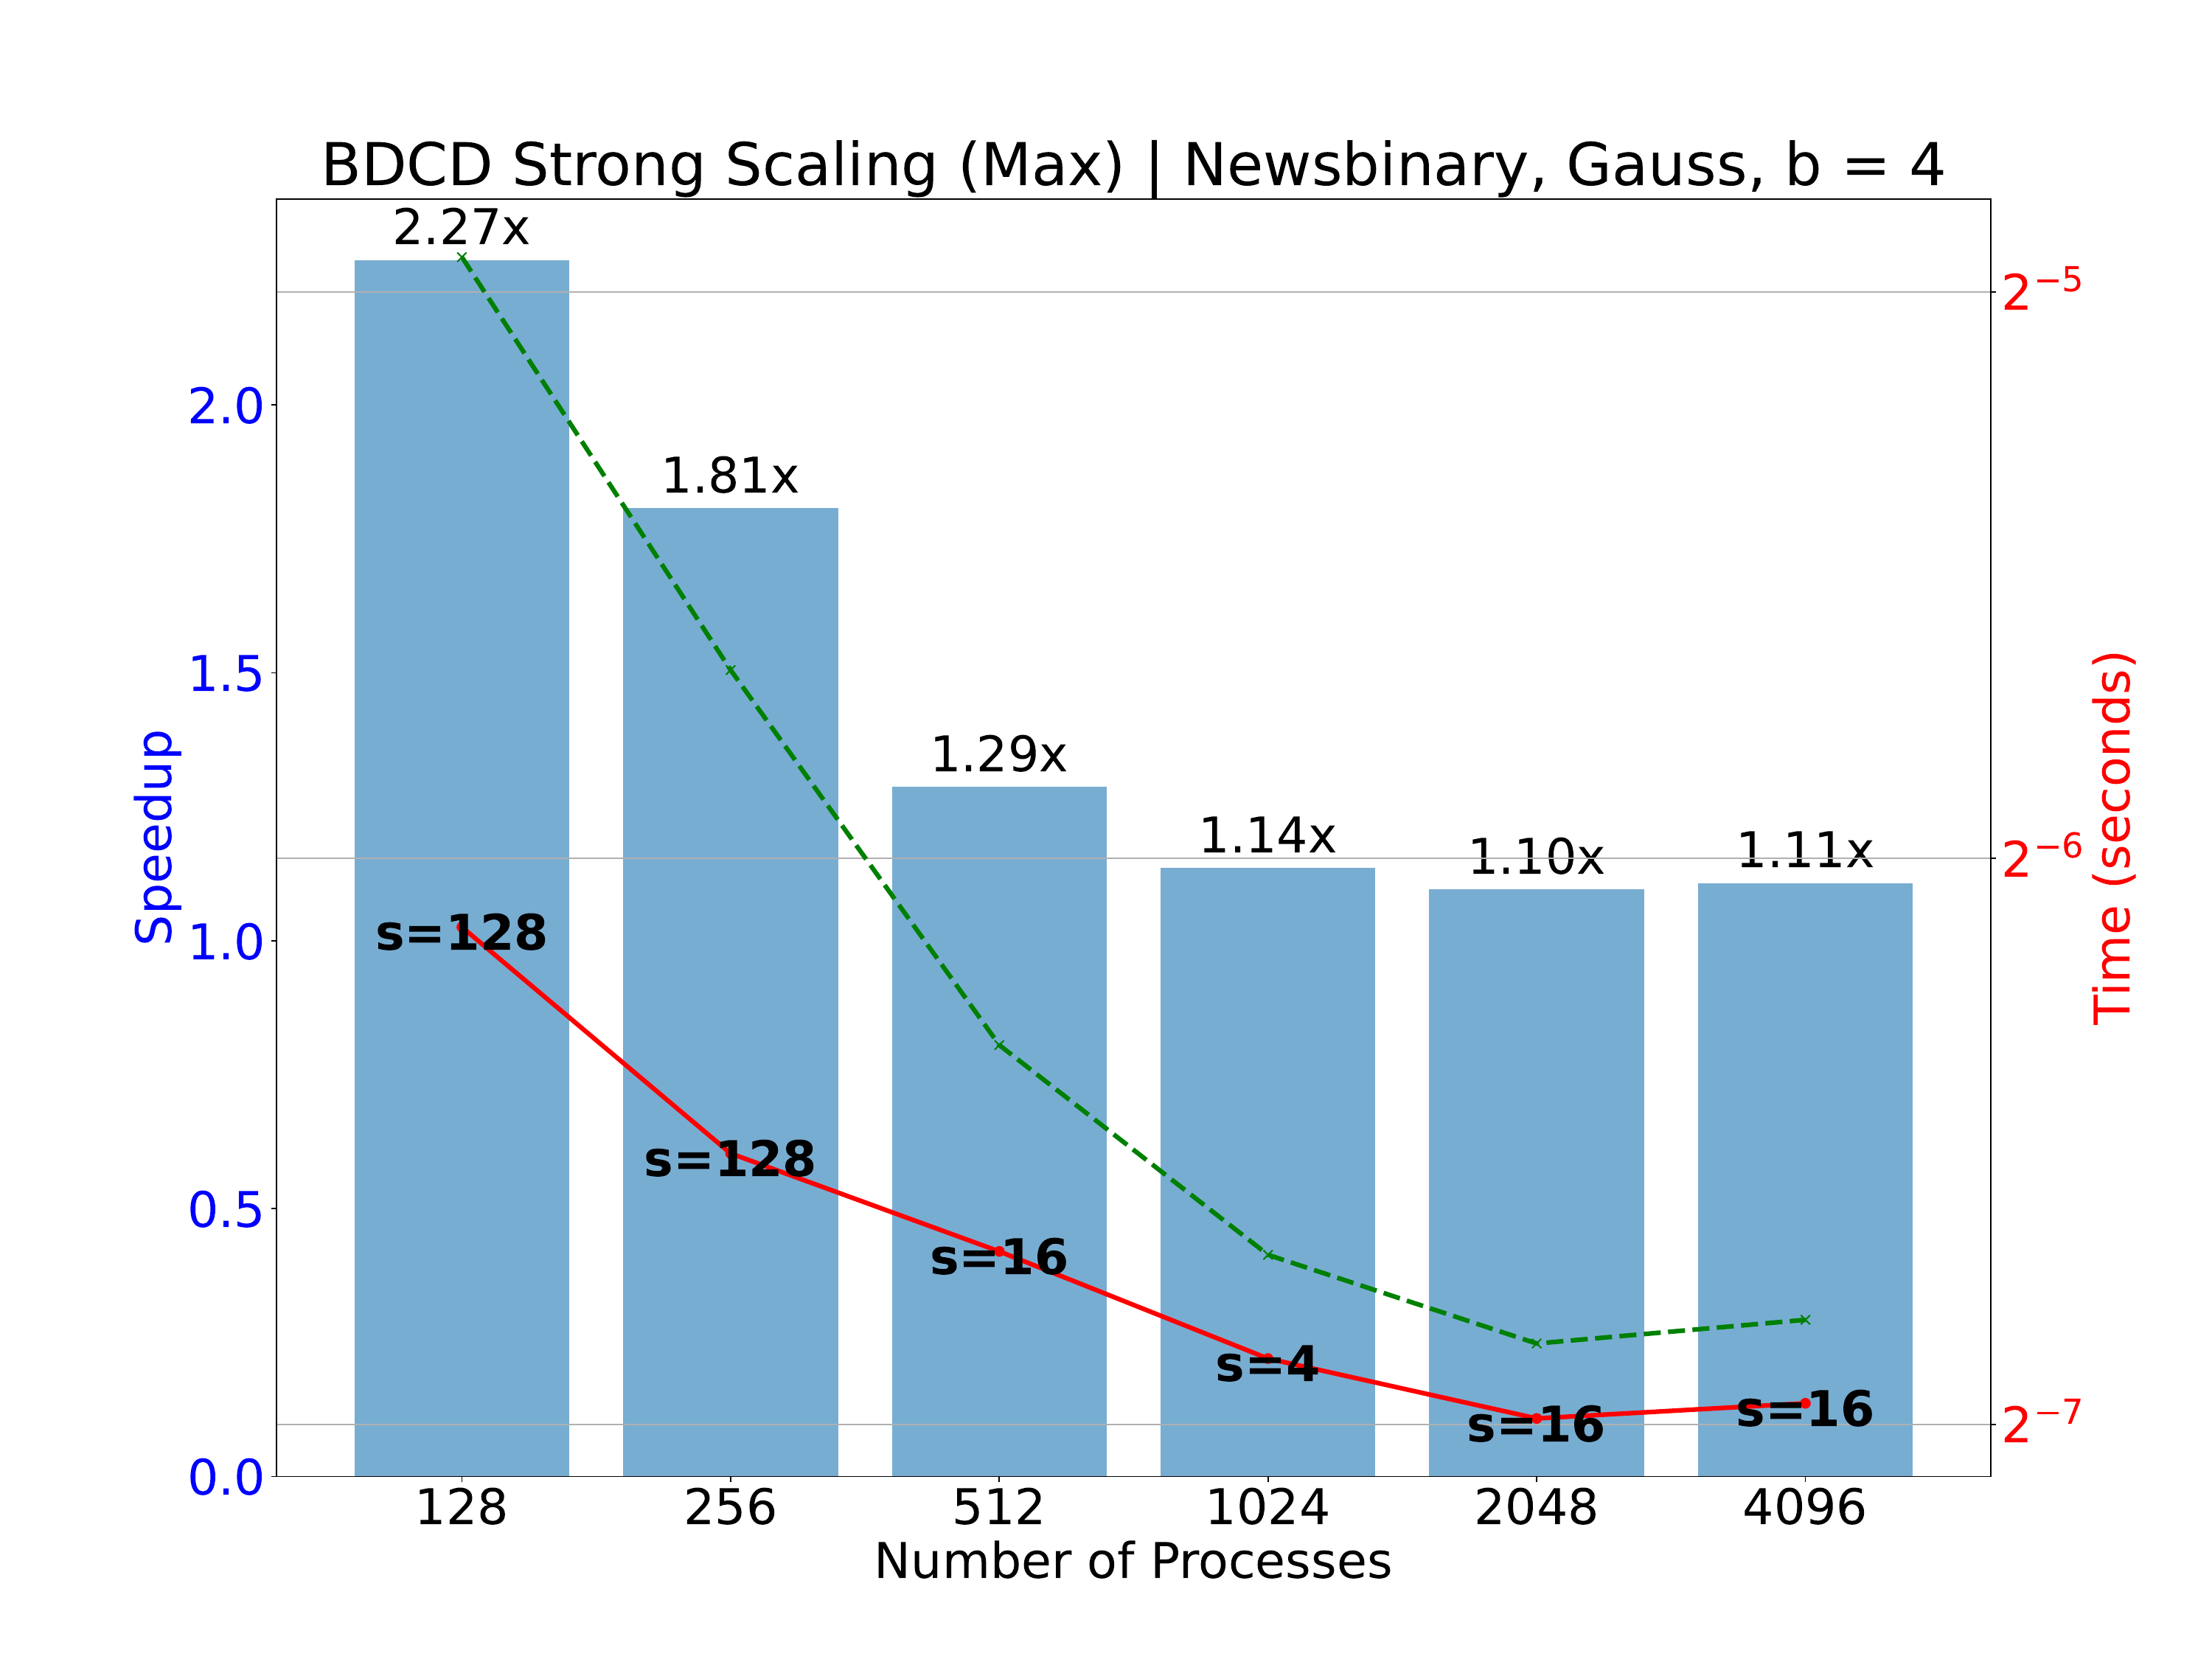}
    \caption{news20.binary, Batch size = 4, gauss}
  \end{subfigure}\hfill

  \caption{Strong Scaling CA-BDCD vs BDCD}
\end{figure*}

\subsubsection{DCD}

\begin{figure*}
  \centering
  \setkeys{Gin}{width=1\linewidth}
  \begin{subfigure}[t]{0.32\textwidth}
    \includegraphics{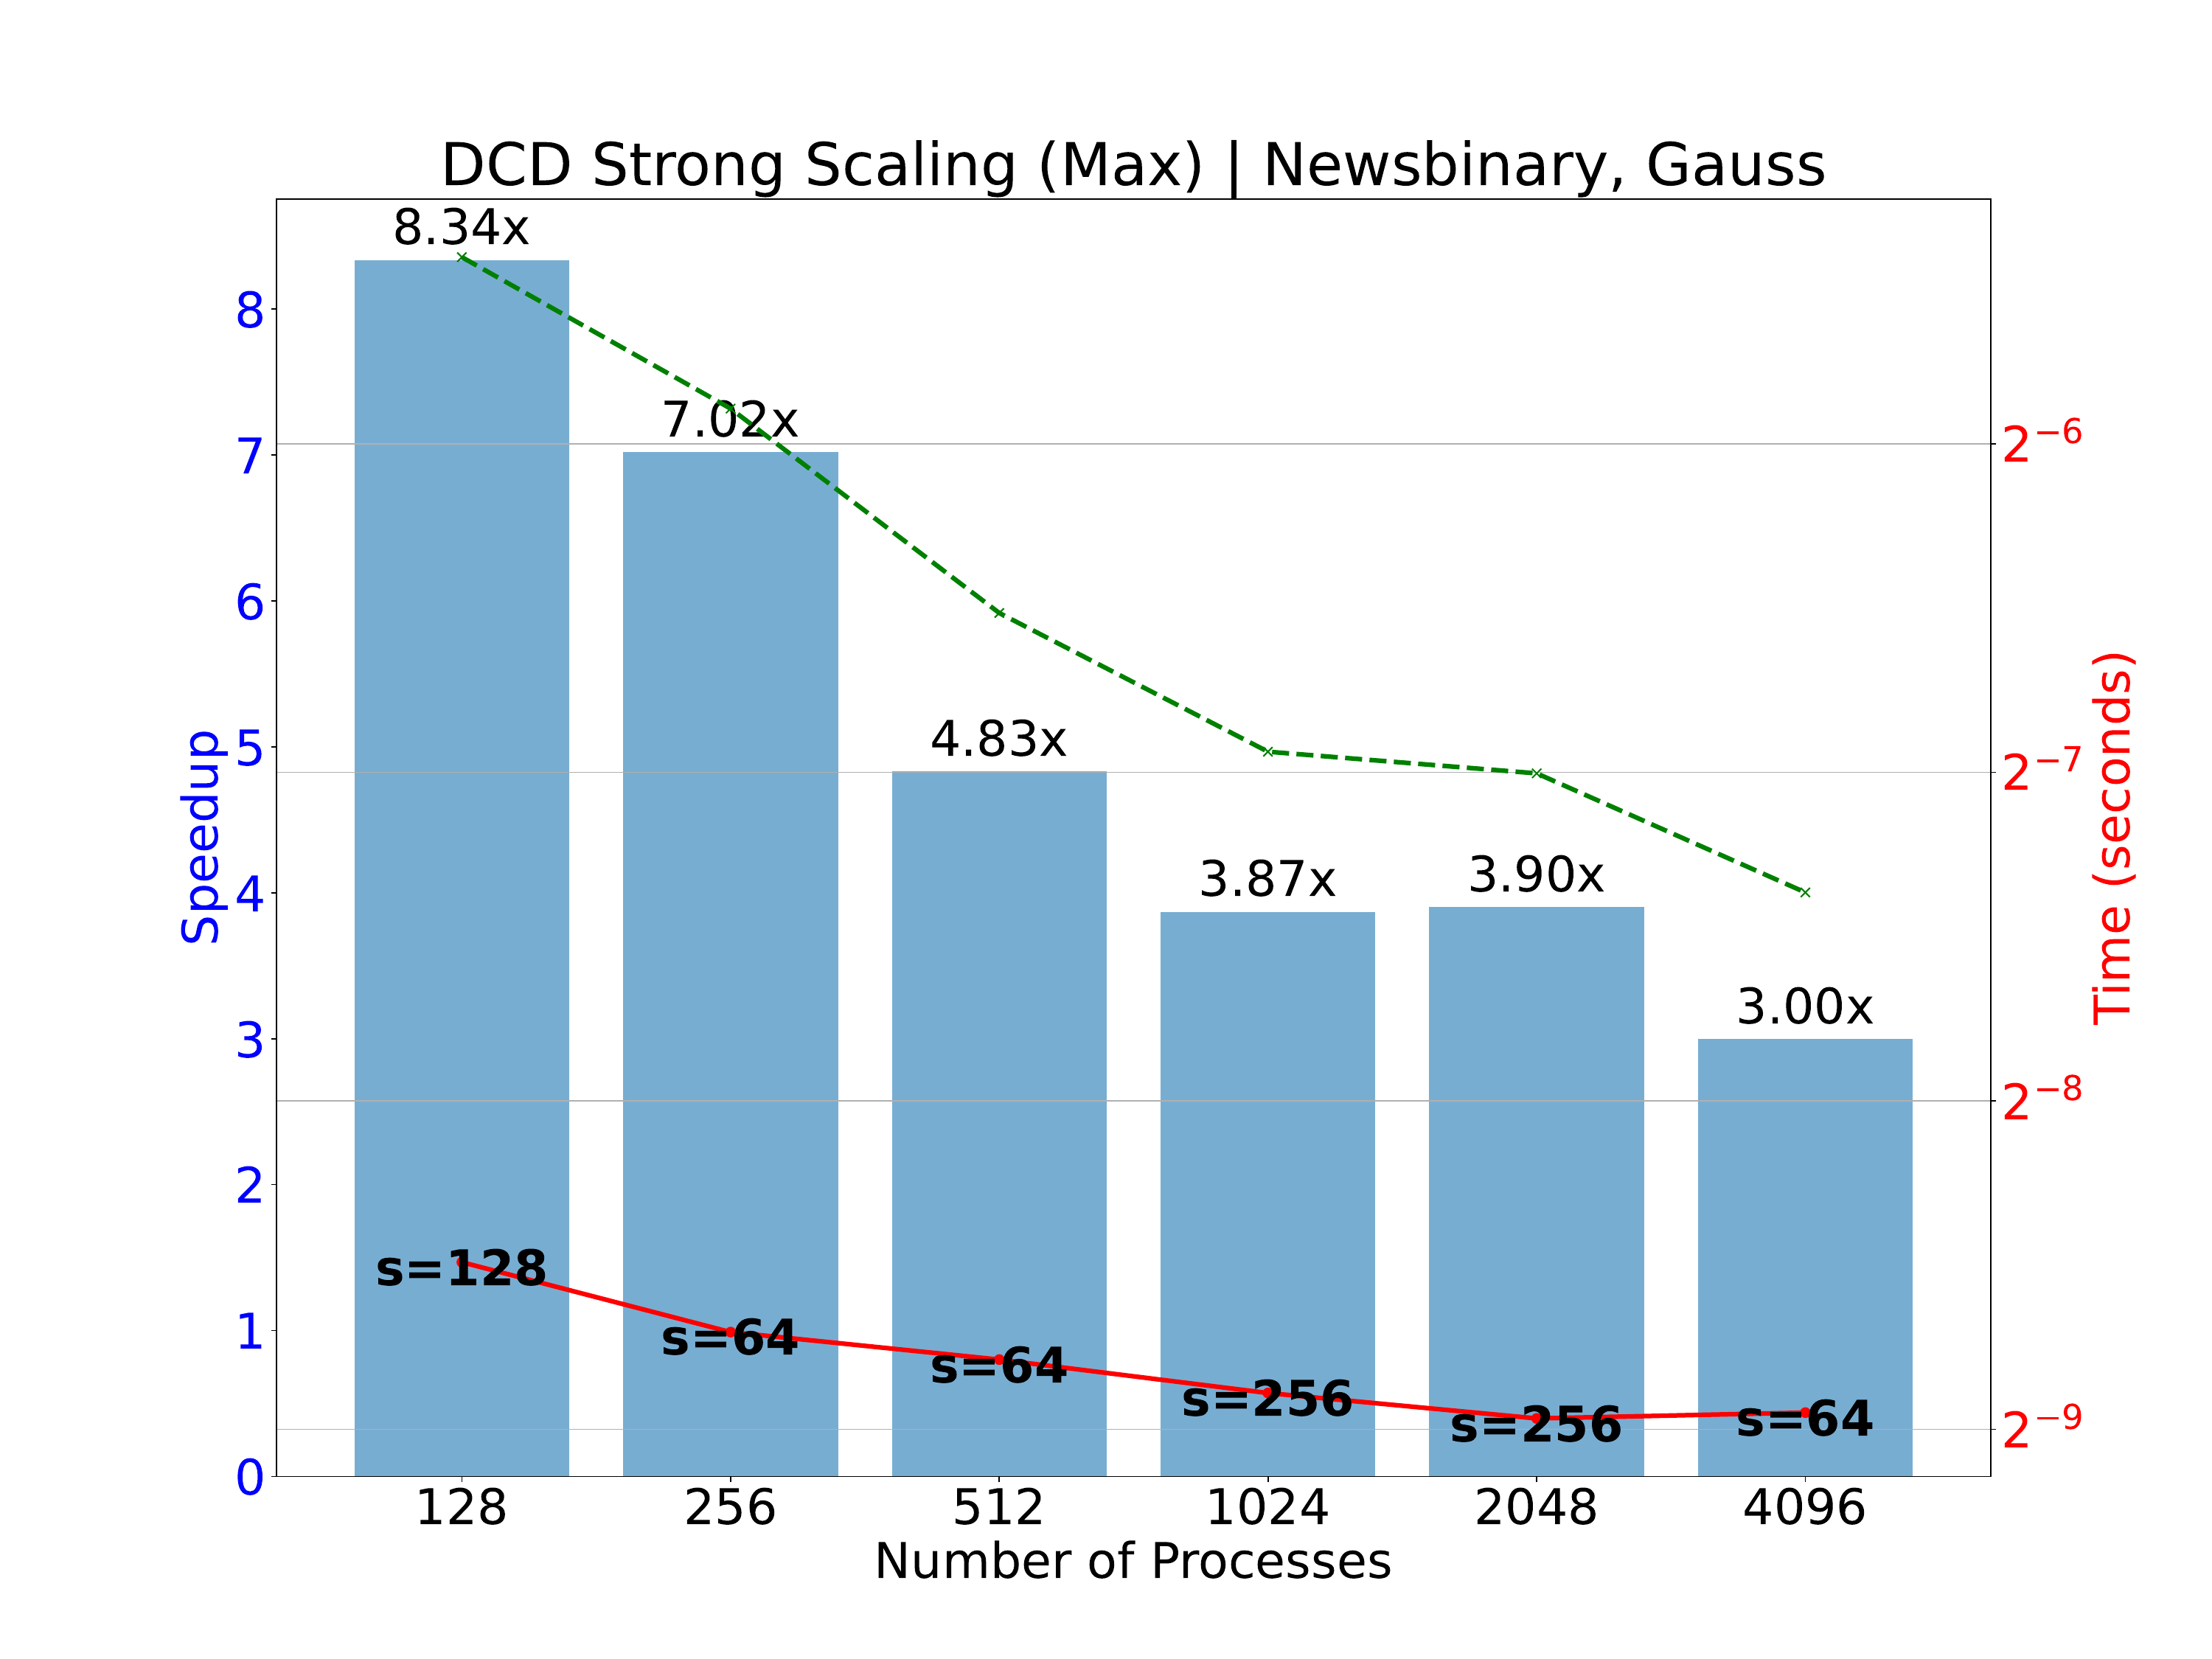}
    \caption{news20.binary, gauss}
  \end{subfigure}\hfill
  \begin{subfigure}[t]{0.32\textwidth}
    \includegraphics{figures/SVM/general/Caksvm_Newsbinary_linear_Max.pdf}
    \caption{news20.binary, linear}
  \end{subfigure}\hfill
  \begin{subfigure}[t]{0.32\textwidth}
    \includegraphics{figures/SVM/general/Caksvm_Newsbinary_poly_Max.pdf}
    \caption{news20.binary, poly}
  \end{subfigure}\hfill

  \caption{Strong Scaling CA-DCD vs DCD, Newsbinary}
\end{figure*}
